# Supplementary material for: Static/Dynamic Filtering for Mesh Geometry
Source: arXiv:1712.03574 ancillary file (2018-03-14)
Supplement: Supplementary file 1 [file SuppMaterial.pdf]

# Static/Dynamic Filtering for Mesh Geometry: Supplementary Material

## 1 Information for Test Data

Below are the vertex and face counts for the mesh models used in the paper:

| Model | Sphere | Cube | Duck | Gargoyle | Armadillo | Knot |
|---|---|---|---|---|---|---|
| Figure No. | 7 | 8 | 12 | 1 | 14 | 9 |
| #Vertices | 30006 | 24578 | 34059 | 50002 | 21582 | 50000 |
| #Faces | 60008 | 49152 | 68114 | 100000 | 43160 | 100000 |
| | | | | | | |
| Model | Merlion | Chinese Lion | Sunflower | Giraffe | Lee Perry Smith | Welsh Dragon |
| Figure No. | 10 | 13 | 16 | 6 | 18 | 15 |
| #Vertices | 283235 | 50003 | 9859 | 14822 | 30549 | 1105352 |
| #Faces | 566465 | 100000 | 15156 | 29628 | 54629 | 2210673 |
| | | | | | | |
| Model | Bunny | Fandisk | Twelve | | | |
| Figure No. | 19 | 19 | 19 | | | |
| #Vertices | 34817 | 6475 | 4610 | | | |
| #Faces | 69630 | 12946 | 9216 | | | |

Table A: Information on the testing mesh normals for SD normal filter.

The Giraffe texture image has $1024 \times 1024$ pixels. The Sunflower texture image has $256 \times 256$ pixels.

## 2 Comparison Between MM Algorithm and Fixed-Point Iteration

We compared the computational time between our fixed-point iteration solver and the MM algorithm, for optimizing the target function $E_{\mathrm{SD}}$. The comparison is preformed using the following test models and parameter settings:

| Model | $\lambda$ | $\eta$ | $\mu$ | $\nu$ |
|---|---|---|---|---|
| Armadillo | 5 | $1.5l_c$ | 2.5 | 0.27 |
| Cube | $1{\cdot}10^4$ | $5l_c$ | 0.8 | 0.2 |
| Duck | 10 | $2l_c$ | 2.5 | 0.3 |
| Knot | $1{\cdot}10^6$ | $4l_c$ | 2.5 | 0.27 |
| Gargoyle | 5 | $3l_c$ | 10 | 0.42 |
| Merlion | 10 | $2.5l_c$ | 20 | 0.26 |

Table B: Test models and parameters for the computational time comparison between the MM algorithm and our fixed-point iteration solver.

For each test model, we ran the MM algorithm for 5 iterations, and our solver for 100 iterations. The MM algorithm were run twice, using Cholesky factorization and Conjugate Gradient to solve the linear system, respectively. All examples are run on a PC with 16GB memory and a quad-core 3.6GHz CPU. Whenever possible, the MM algorithm implementation utilizes OpenMP parallelization. The following table compares the timing and the target energy values for the resulting models:

| Model | #Faces | Method | Initial Energy | Final Energy | Time(s) |
|---|---|---|---|---|---|
| Armadillo | 43K | MM(CG) | 93672.6 | 19679.8 | 7.55 |
| | | MM(Cholesky) | 93672.6 | 19679.8 | 11.08 |
| | | Ours | 93672.6 | 22381.8 | 1.67 |
| Cube | 49K | MM(CG) | $6.30 \cdot 10^7$ | $1.20 \cdot 10^7$ | 74.06 |
| | | MM(Cholesky) | $6.30 \cdot 10^7$ | $1.20 \cdot 10^7$ | 2529.27 |
| | | Ours | $6.30 \cdot 10^7$ | $1.20 \cdot 10^7$ | 18.32 |
| Duck | 68K | MM(CG) | 76113.7 | 16411.5 | 27.80 |
| | | MM(Cholesky) | 76113.7 | 16411.5 | 188.61 |
| | | Ours | 76113.7 | 20946.3 | 4.44 |
| Knot | 100K | MM(CG) | $6.69 \cdot 10^{10}$ | 99999.7 | 318.85 |
| | | MM(Cholesky) | $6.69 \cdot 10^{10}$ | 99999.7 | 2108.65 |
| | | Ours | $6.69 \cdot 10^{10}$ | $1.03 \cdot 10^{10}$ | 43.87 |
| Gargoyle | 100K | MM(CG) | 239660 | 37362 | 40.43 |
| | | MM(Cholesky) | 239660 | 37362 | 283.92 |
| | | Ours | 239660 | 37370.4 | 10.38 |
| Merlion | 566K | MM(CG) | $1.34 \cdot 10^6$ | 166076 | 571.43 |
| | | MM(Cholesky) | – | – | – |
| | | Ours | $1.34 \cdot 10^6$ | 242718 | 62.83 |

Table C: Computational time (in seconds) for our fixed-point iteration solver, and the MM algorithm (using Cholesky factorization and Conjugate Gradient as linear system solver, respectively). The timing for Merlion using MM-Cholesky is not available, because the solver runs out of memory.

# 3 Parameter Settings

## 3.1 Scale-aware filtering

The following table provides the parameter settings for the scale-aware normal filtering examples.

| Parameter | Cube | | | Sphere | |
|---|---|---|---|---|---|
| | Filtered-1 | Filtered-2 | Filtered-3 | Filtered-1 | Filtered-2 |
| $\lambda$ | 500 | 100 | 100 | 100 | 100 |
| $\eta$ | $5\ l_c$ | $6\ l_c$ | $3.5\ l_c$ | $1.2\ l_c$ | $3\ l_c$ |
| $\mu$ | 3 | 20 | 20 | 0.8 | 1.5 |
| $\nu$ | 2 | 0.35 | 0.09 | 0.3 | 0.17 |

Table D: Parameters for scale-aware mesh normal filtering.

## 3.2 Geometry feature enhancement

The following table provides parameters for the geometry feature enhancement results.

| Parameter | Lee | | | Welsh Dragon | | | Gargoyle | | | Armadillo | | |
|---|---|---|---|---|---|---|---|---|---|---|---|---|
| | $M^0$ | $M^1$ | $M^2$ | $M^0$ | $M^1$ | $M^2$ | $M^0$ | $M^1$ | $M^2$ | $M^0$ | $M^1$ | $M^2$ |
| $\lambda$ | 1 | 1 | 500 | 10 | 10 | 10 | 5 | 1.5 | 0.5 | 2 | 1.5 | 1 |
| $\eta$ | $5l_c$ | $3l_c$ | $5\ l_c$ | $7.5l_c$ | $5l_c$ | $2.5l_c$ | $3l_c$ | $2.5l_c$ | $2.5l_c$ | $2.5l_c$ | $1.5l_c$ | $1\ l_c$ |
| $\mu$ | 1.5 | 1.5 | 3 | 20 | 20 | 20 | 10 | 10 | 10 | 1.5 | 1.5 | 1.5 |
| $\nu$ | 0.5 | 0.5 | 2 | 0.35 | 0.35 | 0.35 | 0.42 | 0.3 | 0.3 | 0.45 | 0.33 | 0.23 |

Table E: Parameters for geometry feature enhancement.

### 3.3 Comparison with $\ell_0$ optimization and RGNF

Below are the parameters the comparison between our method and $\ell_0$ optimization and RGNF.

| Method | Parameter | Cube | Knot | Merlion (Bottom) | Merlion (Top) |
|---|---|---|---|---|---|
| $\ell_0$ | $\lambda$ | 5 | 50 | 5 | 5 |
| | $\alpha_0$ | 0.1 | 1 | 0.1 | 0.1 |
| | $\beta_0$ | $1{\cdot}10^{-3}$ | $1{\cdot}10^{-3}$ | $1{\cdot}10^{-3}$ | $1{\cdot}10^{-3}$ |
| | $\mu_\alpha$ | 0.5 | 0.5 | 0.5 | 0.5 |
| | $\mu$ | 1.414 | 1.414 | 1.414 | 1.414 |
| | $\beta_{max}$ | $1{\cdot}10^{4}$ | $1{\cdot}10^{4}$ | $5{\cdot}10^{3}$ | 200 |
| RGNF | $\sigma_s$ | 8 | 5 | 5 | 5 |
| | $\sigma_r$ | 0.1 | 0.35 | 0.6 | 0.1 |
| | $N_{\text{iter}}$ | 5 | 5 | 5 | 5 |
| Ours | $\lambda$ | $1{\cdot}10^{6}$ | 10 | 100 | $1{\cdot}10^{4}$ |
| | $\eta$ | $5l_c$ | $2l_c$ | $2l_c$ | $3l_c$ |
| | $\mu$ | 2.5 | 2.5 | 2 | 20 |
| | $\nu$ | 0.4 | 0.8 | 0.23 | 0.12 |

Table F: Parameters for the comparison between SD filtering, $\ell_0$ optimization, and RGNF.

### 3.4 Texture image filtering

The following tables parameter settings for texture image filtering results.

| Parameter | Sunflower | | | Giraffe | |
|---|---|---|---|---|---|
| | $T^0$ | $T^1$ | $T^2$ | Filtered-1 | Filtered-2 |
| $\lambda$ | 100 | 100 | 100 | 10 | 10 |
| $\eta$ | $1l_c$ | $0.28l_c$ | $0.20l_c$ | $1l_c$ | $1l_c$ |
| $\mu$ | 0.2 | 0.2 | 0.2 | 0.2 | 0.2 |
| $\nu$ | 0.15 | 0.15 | 0.15 | 0.1 | 0.08 |

Table G: Parameters for texture image filtering.

### 3.5 Mesh denoising

Below are the parameters for mesh denoising examples.

| Method | Parameter | Bunny | Fandisk | Twelve |
|---|---|---|---|---|
| GMNF | $r$ | 2.0(2.7×) | 2.0(2.6×) | 2.0(2.6×) |
| | $\sigma_{\text{r}}$ | 0.55 | 0.30 | 0.27 |
| | $k_{\text{iter}}$ | 4 | 50 | 75 |
| | $v_{\text{iter}}$ | 4 | 20 | 20 |
| Ours | $\lambda$ | 100 | 100 | 250 |
| | $\eta$ | $0.4l_c$ | $0.7l_c$ | $1.5l_c$ |
| | $\mu$ | 20 | 20 | 60 |
| | $\nu$ | 0.3 | 0.27 | 0.28 |
| | $W_{\text{closeness}}$ | 2.5 | 0.6 | 2 |
| | $k_{\text{iter}}$ | 20 | 50 | 20 |
| | $v_{\text{iter}}$ | 5 | 10 | 100 |

Table H: Parameters for mesh denoising.

### 3.6 Explanation of parameters

- $\ell_0$ [1] (Table F):
  - $\lambda$: weight for the $L_0$ term in the target function.
  - $\beta_0$: initial weight for the differential term.
  - $\mu$: it is the speed at increasing $\beta$.
  - $\beta_{max}$: max weight for the differential term.
  - $\alpha_0$: initial weight for the regular term.
  - $\mu_\alpha$: it is the speed at decreasing $\alpha$.
- RGNF [3] (Table F):
  - $\sigma_s$: it is related to the scale size of geometry features.
  - $\sigma_r$: it is related to the desired smoothness of the final results.
  - $N_{\text{iter}}$: number of iterations for updating normals.
- GMNF [4] (Table H):
  - $r$: radius for the geometrical neighborhood, also shown as the ratio with respect to the average distance between neighboring face centroids; not applicable if a topological neighborhood is used.
  - $\sigma_{\text{r}}$: variance of the range kernel.
  - $k_{\text{iter}}$: number of iterations for updating normals.
  - $v_{\text{iter}}$:number of iterations for a vertex update.
- Ours (Tables B, D, E, F, G, H) :
  - $\lambda$: it controls the scale of the preserved geometry features.
  - $\eta$: it controls the neighborhood size.
  - $\mu$: it controls the desired smoothness.
  - $\nu$: it controls the desired filter scale.
  - $k_{\text{iter}}$: number of iterations for updating vertex position from filtered normals.
  - $v_{\text{iter}}$: number of times for performing SD normal filter.

# 4 Convergence of Fixed-Point Iteration

In this section, we prove that the fixed-point iteration without normalization (Equation (13) in the paper) is guaranteed to convergence to a local minimum of the target function $E_{\text{SD}}$ (Equation (4) in the paper). Note that each fixed-point iteration is a single step of Jacobi iteration for the linear system that minimizes the following majorization function

$$F^k(\mathbf{N}) = \sum_{i=1}^{3} \Big( (\mathbf{N}_i - \hat{\mathbf{N}}_i)^T \mathbf{D} (\mathbf{N}_i - \hat{\mathbf{N}}_i) + \lambda \mathbf{N}_i^T \mathbf{M}^k \mathbf{N}_i \Big),$$

where $\mathbf{N}_i$ $(i = 1, 2, 3)$ are vectors that collect the $x$-, $y$-, and $z$-coordinates of the face normal variables, and $\hat{\mathbf{N}}_i$ are their values on the input mesh. The matrix $\mathbf{N}^k$ is determined from the current variable values $\mathbf{N}^k$, and the matrix $\mathbf{D} + \lambda \mathbf{M}^k$ is symmetric positive and diagonally dominant. We will prove the following

**Proposition 1.** *The fixed-point iteration produces new variable values $\mathbf{N}^{k+1}$ for which $F^k(\mathbf{N}^{k+1}) < F^k(\mathbf{N}^k)$, unless $\mathbf{N}^k$ is the minimum of $F^k$ in which case $\mathbf{N}^{k+1} = \mathbf{N}^k$.*

Note that $F^k(\mathbf{N}) \geq E_{\text{SD}}(\mathbf{N})$ for all $\mathbf{N}$, and $F^k(\mathbf{N}^k) = E_{\text{SD}}(\mathbf{N}^k)$. Moreover, if $\mathbf{N}^k$ is a minimum of $F^k$, then it is also a local minimum of $E_{\text{SD}}$ [2]. Therefore, we have $E_{\text{SD}}(\mathbf{N}^k) \leq F^k(\mathbf{N}^k) < F^k(\mathbf{N}^k) = E_{\text{SD}}(\mathbf{N}_k)$, unless $\mathbf{N}_k$ is local minimum of $E_{\text{SD}}$ in which case $\mathbf{N}^{k+1} = \mathbf{N}^k$. In other words, the fixed-point iteration is guaranteed to decrease the target function $E_{\text{SD}}$ until it converges to a local minimum of $E_{\text{SD}}$.

We prove Proposition 1 by showing that a single step of the Jacobi iteration

$$\mathbf{N}^{k+1} = \mathbf{Q}^{-1}(\mathbf{D}\hat{\mathbf{N}} - \mathbf{R}\mathbf{N}^k)$$

is guaranteed to decrease $F^k$ unless $\mathbf{N}^k$ is the minimum. Here $\mathbf{Q}$ and $\mathbf{R}$ are the diagonal and off-diagonal parts of the matrix $\mathbf{D} + \lambda\mathbf{M}^k$ respectively, such that $\mathbf{D} + \lambda\mathbf{M}^k = \mathbf{Q} + \mathbf{R}$. Our proof is inspired by a post from StackExchange user Hui Zhang [1]. First, we denote the minimum of $F^k$ by

$$\mathbf{N}^* = (\mathbf{D} + \lambda\mathbf{M}^k)^{-1}\mathbf{D}\hat{\mathbf{N}},$$

and let

$$\mathbf{P}^k = \mathbf{N}^{k+1} - \mathbf{N}^k, \quad \mathbf{E}^k = \mathbf{N}^* - \mathbf{N}^k.$$

Then we have

$$\begin{aligned}\mathbf{Q}^{-1}(\mathbf{D} + \lambda\mathbf{M}^k)\mathbf{E}^k &= \mathbf{Q}^{-1}(\mathbf{D} + \lambda\mathbf{M}^k)(\mathbf{N}^* - \mathbf{N}^k) = \mathbf{Q}^{-1}(\mathbf{D}\hat{\mathbf{N}} - (\mathbf{D} + \lambda\mathbf{M}^k)\mathbf{N}^k) \\ &= \mathbf{Q}^{-1}(\mathbf{D}\hat{\mathbf{N}} - (\mathbf{Q} + \mathbf{R})\mathbf{N}^k) = \mathbf{Q}^{-1}(\mathbf{D}\hat{\mathbf{N}} - \mathbf{R}\mathbf{N}^k) - \mathbf{Q}^{-1}\mathbf{Q}\mathbf{N}^k \\ &= \mathbf{N}^{k+1} - \mathbf{N}^k = \mathbf{P}^k.\end{aligned}$$

Therefore, when $\mathbf{N}^k$ is the minimum of $F^k$, we have $\mathbf{E}^k = \mathbf{0}$ and as a result $\mathbf{N}^{k+1} - \mathbf{N}^k = \mathbf{0}$. If $\mathbf{N}^k$ is not the minimum of $F^k$, then the above formula indicates that $\mathbf{P}^k \neq \mathbf{0}$ we denote $\mathbf{K} = \mathbf{D} + \lambda\mathbf{M}^k$, then

$$\begin{aligned}& F^k(\mathbf{N}^{k+1}) - F^k(\mathbf{N}^k) \\ = & \sum_{i=1}^{3} -2(\mathbf{N}_i^{k+1} - \mathbf{N}_i^k)^T\mathbf{D}\hat{\mathbf{N}}_i + (\mathbf{N}_i^{k+1} - \mathbf{N}_i^k)^T\mathbf{K}(\mathbf{N}_i^{k+1} - \mathbf{N}_i^k) + 2(\mathbf{N}_i^{k+1} - \mathbf{N}_i^k)^T\mathbf{K}\mathbf{N}_i^k \\ = & \sum_{i=1}^{3} -2(\mathbf{P}_i^k)^T\mathbf{K}\mathbf{N}_i^* + (\mathbf{P}_i^k)^T\mathbf{K}\mathbf{P}_i^k + 2(\mathbf{P}_i^k)^T\mathbf{K}\mathbf{N}_i^k = \sum_{i=1}^{3}(\mathbf{P}_i^k)^T\mathbf{K}\mathbf{P}_i^k - 2(\mathbf{P}_i^k)^T\mathbf{K}\mathbf{E}_i^k \\ = & \sum_{i=1}^{3}(\mathbf{P}_i^k)^T\mathbf{K}\mathbf{P}_i^k - 2(\mathbf{P}_i^k)^T\mathbf{Q}\mathbf{P}_i^k = \sum_{i=1}^{3}(\mathbf{P}_i^k)^T(\mathbf{K} - 2\mathbf{Q})\mathbf{P}_i^k,\end{aligned}$$

where $\mathbf{E}_i^k, \mathbf{P}_i^k$ denotes the columns of $\mathbf{E}^k, \mathbf{P}^k$, respectively. Note that the off-diagonal elements of $K$ are non-negative, while the diagonal elements of $K$ are all positive, and $K$ is diagonally dominant. Therefore, with $\mathbf{Q}$ being the diagonal part of $\mathbf{K}$, matrix $\mathbf{K} - 2\mathbf{Q}$ is negative definite. And with $\mathbf{P}^k \neq 0$, we have $\sum_{i=1}^{3}(\mathbf{P}_i^k)^T(\mathbf{K} - 2\mathbf{Q})\mathbf{P}_i^k < 0$, meaning that $F^k(\mathbf{N}^{k+1}) < F^k(\mathbf{N}^k)$.

# References


[1] Lei He and Scott Schaefer. Mesh denoising via $L_0$ minimization. *ACM Trans. Graph.*, 32(4):64:1–64:8, 2013.

[2] Kenneth Lange. *MM Optimization Algorithms*. SIAM, 2016.

[3] Peng-Shuai Wang, Xiao-Ming Fu, Yang Liu, Xin Tong, Shi-Lin Liu, and Baining Guo. Rolling guidance normal filter for geometric processing. *ACM Trans. Graph.*, 34(6):173, 2015.

[4] Wangyu Zhang, Bailin Deng, Juyong Zhang, Sofien Bouaziz, and Ligang Liu. Guided mesh normal filtering. *Comput. Graph. Forum*, 34(7):23–34, 2015.


[1] `https://scicomp.stackexchange.com/questions/1478/jacobi-iteration-to-reduce-the-quadratic-function`
